# Supplementary material for: Initial solidification dynamics of spreading droplets
Source: arXiv:2005.12189 source file (2020-05-26)
Supplement: Supplementary file 1 [file SuppMat-min.pdf]

**INITIAL SOLIDIFICATION DYNAMICS OF SPREADING DROPLETS**

**SUPPLEMENTARY MATERIALS**

**Experimental setup**

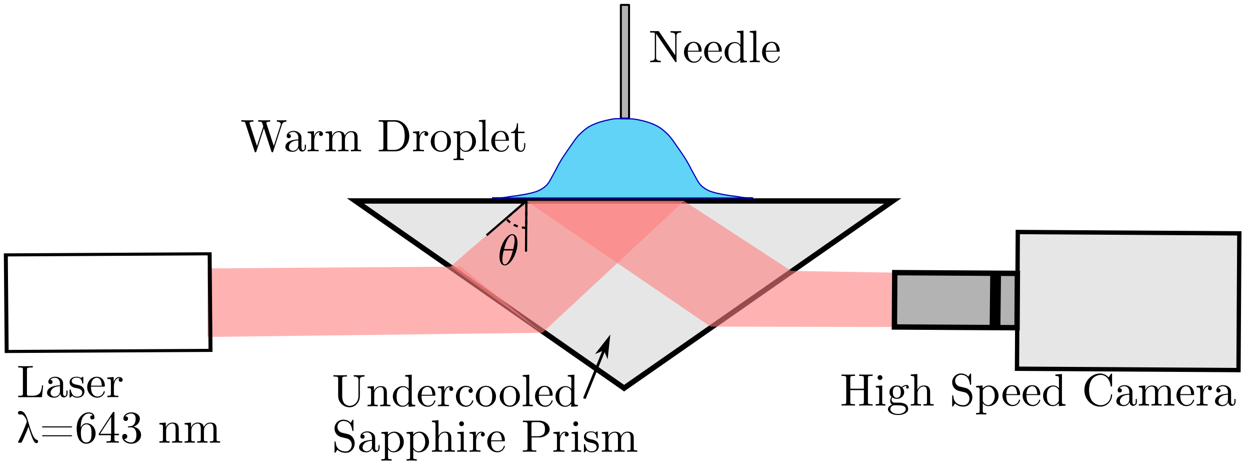


FIG. 1. Schematic of the TIR setup.

The experimental setup is depicted in figure 1. A hexadecane droplet ($C_{16}H_{34}$, Sigma-Aldrich, thermal properties in table I), with freezing point $T_f = 18\,°\mathrm{C}$, is formed at the end of a needle (Nordson EFD, with inner diameter $d_i = 0.33$ mm). This needle is fed by a syringe pump (Harvard PHD2000), resulting in a droplet diameter of $D_0 = 1.7 \pm 0.1$ mm. The hexadecane is slightly heated to an initial droplet temperature of $T_0 = 37\,°\mathrm{C}$ to prevent solidification in the needle. This heating has no significant influence on the spreading behavior [1]. The droplet is gently deposited onto a sapphire prism (Crystan ltd.), which is cooled below the freezing temperature of the droplet. The thermal properties of the prism are given in table I The prism is placed in an aluminum holder, that is PID-controlled at a fixed temperature ranging from 8 °C to 20 °C. Before each spreading event the substrate temperature of the sapphire prism is measured with an NTC-type thermistor (Wavelength Electronics). We record the bottom view with a high-speed camera (Photron FastCam SA-X2) equipped with a long distance microscope (Navitar 12x Telecentric zoom system) at recording rates from 20000 fps to 30000 fps and a spatial resolution of $9\,\mu\mathrm{m\,pixel}^{-1}$. In order to discriminate between the solidified, wetted and dry areas we employ TIR imaging

[2]. The substrate is illuminated under an angle $\theta$ by a 60 mW laser (wavelength 643 nm) expanded to about 20 mm diameter and introduced into the prism via mirrors.

**Material properties**

TABLE I. Material properties of the liquid hexadecane and sapphire prism

| Material | Hexadecane (droplet) | Sapphire (prism) |
|---|---|---|
| Density $\rho$ (kilogram/m$^3$) | 770 | 3980 |
| Thermal Conductivity k (watt/m/K) | 0.15 | 34.6 |
| Heat capacity $c_p$ (joule/kg/K) | 2310 | 761 |
| Surface tension $\sigma$ (newton/m) | 0.028 | - |
| Viscosity $\eta$ (pascals) | 0.003 | - |

**Visualisation**

Here we explain more details of the TIR imaging method employed to visualize the solidification processes. This method has the advantage to be only sensitive to measure processes in a thickness smaller than the first micrometer of the droplet. Illuminating the bottom of the prism is achieved by using a monochromatic light source. We use a 643 nm diode laser, which is expanded by a set of lenses, to have the complete footprint of the drop illuminated. The camera records the reflected light through the other side of the prism.

The incident angle $\theta$ should be larger than the critical angle $\theta_c = \sin^{-1}(n_2/n_1)$ for the TIR imaging to work. Here $n_2$ is the refractive index of the sapphire prism and $n_1$ that of the medium across the interface. The image of the droplet is distorted to an ellipse, back transformation and angles of incidence are obtained as described in Ref. [2]. In this Letter, only reconstructed images are shown. In earlier work, for heated surfaces [3], $\alpha$ was chosen to be larger than $\theta_c$, using $n_1 = 1$ for air, but smaller than $n_2$ for the liquid. This results in TIR for locations that are dry, resulting in a white spot on the camera and normal refraction according to the Fresnel equations for the wetted areas, resulting in the loss of intensity on the camera.

In the present study however, we operate the setup for $\alpha$ being smaller than $\theta_c$ for *both* air and the liquid. As a consequence light is refracted everywhere, except where the refractive index makes a sudden jump. This jump can both come from the sudden change from air to liquid or from fluctuations in the refractive index as a result of amorphous solid patches. Both cases result in diffraction of the evanescent wave on the other side of the prism interface. It is this diffraction which enables us to observe the moving contact line as well as the solidified areas in the drop.

A simulation of a contact line is shown in figure , where a Gaussian beam is propagating from right to left and is reflected on the prism surface. The simulations solve the time independent Helmholtz-equation in the three media, using the code developed by Osnabrugge et. al. [4]. The domain is normalized by the incident wave length $\lambda$ and the beam width is $10\lambda$. The prism material has a refractive index of $n = 1.45$; and $n = 1$ is used on the right, for the air, whereas $n = 1.33$ is used for the liquid part. The resulting normalized electric field is represented by the color between zero (blue) and 1 (yellow). The inset magnifies the details at the contact line. The difference in decay length $d = \lambda_0/(4\pi n_1)\left(\sin^2\theta - (n_2/n_1)^2\right)^{-1/2}$ for the glass-air and glass-liquid interfaces results in the intensity fluctuations in the right part of the glass domain. However, the finite aperture of optical systems used in experiments cannot resolve this small scale feature. The diffraction pattern captured is used to identify the contact line position.

**Nucleation rate**

The nucleation rate can be expressed as an Arrhenius type reaction velocity:

$$J_0 = A \exp \frac{-E_a}{k_B T_f}, \tag{1}$$

where $J_0$ is the nucleation rate, $k_B$ the Boltzmann constant, and $A$ the attempt frequency. $E_a$ is a critical activation energy to form a stable nucleus. The formation of a stable crystalline phase in an under-cooled liquid is controlled by the local free energy barrier. The activation energy associated with nucleation, assuming the nucleus is a sphere, is given by $E_a = (16\pi/3)\,\gamma_{ls}^3 f\left(\theta_{ls}\right)/\left(\Delta g\right)^2$, where $\Delta g = \Delta S_{fus}\Delta T$ is the free energy difference between the liquid and solid phase and $\gamma_{ls} = 0.0068\,\mathrm{J\,m^{-2}}$[5] is the interfacial tension between the two phases. The entropy of fusion is $\Delta S_{fus} = 6.28\cdot 10^5\,\mathrm{J\,m^{-3}\,K^{-1}}$ [6]. For a spherical particle on

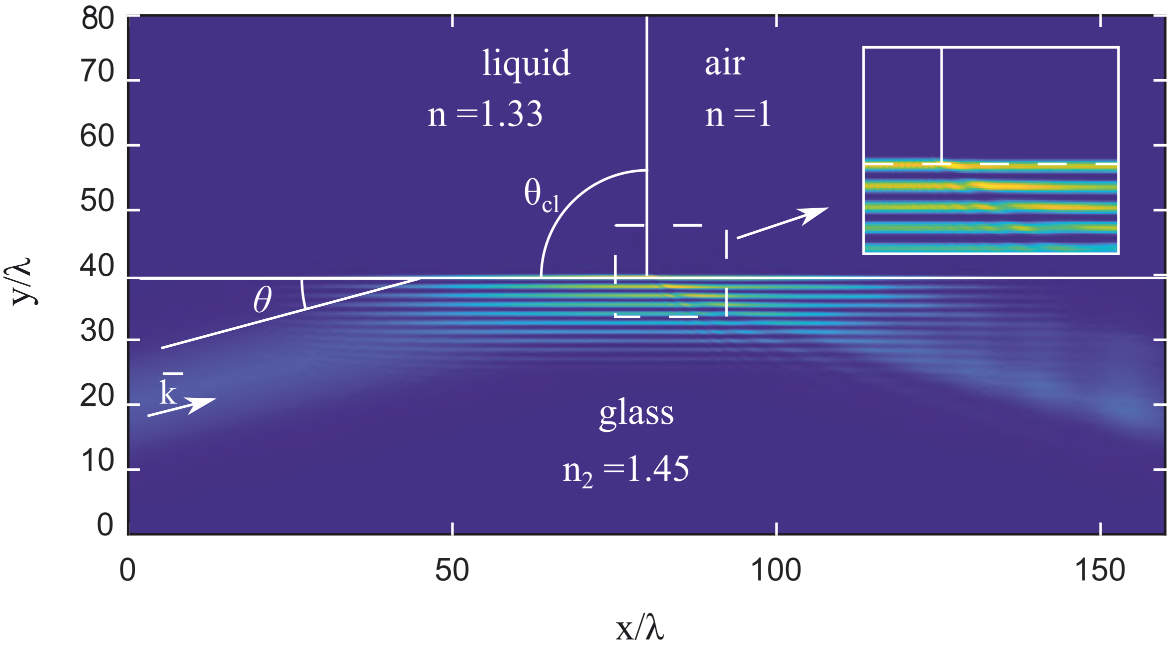


FIG. 2. Simulation results, showing the normalized intensity field of a collimated laser beam of width 10 $\lambda$. The wave vector $\vec{k}$, which determines the incident angle $\theta$ with the glass surface, is chosen such that the light undergoes total internal reflection for both the liquid (left) and air (right) phases. The vertical white line represents the liquid-air interface, whereas the inset reveals the details at the contact line, showing the diffraction patterns leading to the visibility of the contact line.

a foreign surface, $f(\theta_{ls}) = 1/4(2 + \cos\theta_{ls})(1 - \cos\theta_{ls})^2$ is the geometrical correction factor, where $\theta_{ls}$ is the contact angle between a solid nucleus and the liquid phase surrounding it with the substrate [7]. This correction factor is determined by the change in volume and surface area between a spherical nucleus and a spherical cap on a surface. It expresses the difference in the energy barrier when heterogeneous nucleation takes place, which occurs for sessile droplets [8]. The nucleation behavior of spreading droplets is not yet known, as far as the authors are aware. The attempt frequency $A$ is proportional to the characteristic frequency of molecular motion [6, 9, 10], $A = C\sqrt{\frac{\gamma_{ls}}{k_B T_{prism}}}\alpha\frac{\mathcal{D}}{d^2}$. Here C is a numerical constant set to 1.65 [11], $\alpha$, $d$ and $\mathcal{D} = (k_B T_{prism})\,/\,(3\pi\eta d)$ are the molecular number density, molecular diameter and the Stokes-Einstein diffusion constant of hexadecane in its liquid phase.

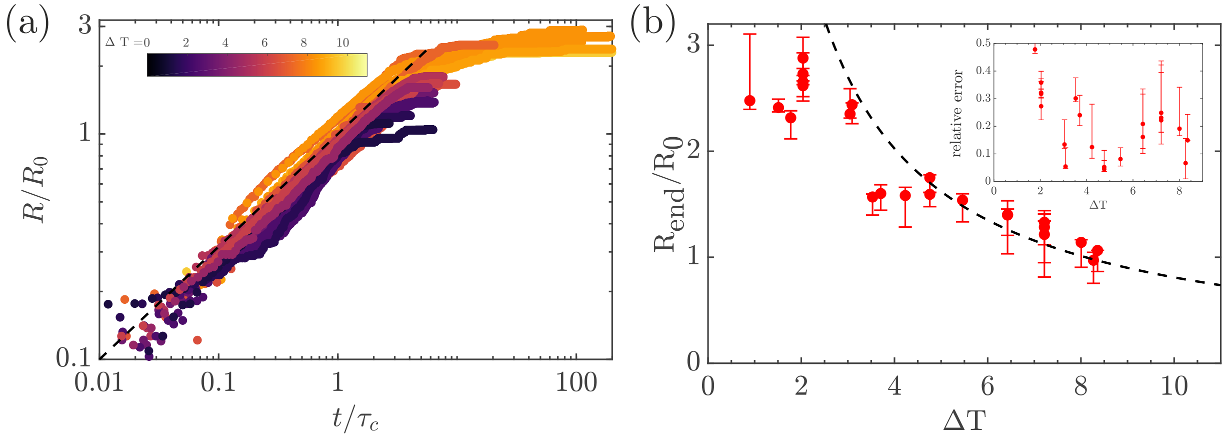


FIG. 3. (a) Spreading radius versus time for a range of substrate temperatures, with ——the inertial scaling $\propto t^{1/2}$, Equation (2). (b) Radius of arrest versus temperature. - - -is the model of equation (3). The error bars show the minimum and maximum radius of a single arrest event. For $\Delta T < 3\,\mathrm{K}$, the model is not valid. The inset shows the relative error $\left|\left(R_{th} - R_{exp}\right)/R_{th}\right|$

**Droplet spreading**

Here we show the extent of hexadecane spreading on a sapphire substrate, including the maximum spreading radius. Side view images are obtained using a high speed camera (FASTCAM-APX RS) fitted with a macro lens at 10000 fps, with a spatial resolution of $18\,\mathrm{\mu m\,pixel^{-1}}$, where the initial frame is synchronized with the bottom view. For substrate temperatures above the freezing temperature, the isothermal spreading laws are recovered, figure 3, as was reported for the spreading of hexadecane droplets on copper [1]. Initially,

$$\frac{R}{R_0} \propto \left(t/\tau_c\right)^{1/2}, \tag{2}$$

with the spreading radius $R(t)$, droplet radius $R_0$, and the capillary time $\tau_c = (\rho R_0^3/\sigma)^{1/2}$ [12–15]. At later stages, the spreading resembles Tanner's law $R/R_0 \propto \left(\sigma t/\eta R_0\right)^{1/10}$ for the spreading of a small viscous drop [16]. For $T < T_\mathrm{f}$, the contact line is arrested due to solidification. Figure 3b shows the mean arrest radius $R_{end}$ as a function of the under-cooling. For $\Delta T > 3.5\,\mathrm{K}$, they follow the criterium of Ref.[1]:

$$\frac{R_{end}}{R_0} \propto \frac{R_0}{\tau_c \mu \Delta T}, \tag{3}$$

where $\mu$ is the kinetic under-cooling coefficient. The best fit to this equation for our data was found with a prefactor of 0.18. This leads to a typical error $|(R_{th} - R_{exp})/R_{th}| < 20\%$, the theoretical radius $R_{th}$ and the measured radius $R_{exp}$ for undercooling $\Delta T > 3$K, see the inset in figure 3b. Nucleation at the contact line is not distributed evenly, therefore the arrested droplets are not constant in radius, which is shown by the error bars in figure 3b.


[1] R. De Ruiter, P. Colinet, P. Brunet, J. H. Snoeijer, and H. Gelderblom, Phys. Rev. Fluids **2**, 043602 (2017).

[2] M. Shirota, M. A. van Limbeek, D. Lohse, and C. Sun, Eur. Phys. J. E **40**, 54 (2017).

[3] M. A. Van Limbeek, M. Shirota, P. Sleutel, C. Sun, A. Prosperetti, and D. Lohse, Int. J. Heat Mass Transf. **97**, 101 (2016).

[4] G. Osnabrugge, S. Leedumrongwatthanakun, and I. M. Vellekoop, J. Comput. Phys. **322**, 113 (2016).

[5] M. J. Oliver and P. D. Calvert, J. Cryst. Growth **30**, 343 (1975).

[6] A. B. Herhold, D. Ertaş, A. J. Levine, and H. E. King, Phys. Rev. E - Stat. Physics, Plasmas, Fluids, Relat. Interdiscip. Top. **59**, 6946 (1999).

[7] J. Mullin, *Org. Process Res. Dev.*, 4th ed., Vol. 6 (Butterworth-Heinemann, Oxford, 2007) pp. 201–202.

[8] M. Dorrestijn, S. Jung, C. M. Megaridis, D. Raps, A. Das, and D. Poulikakos, Langmuir **27**, 3059 (2011).

[9] D. T. Wu, Solid State Phys. **50**, 37 (1996).

[10] A. B. Herhold, H. E. King, and E. B. Sirota, J. Chem. Phys. **116**, 9036 (2002).

[11] K. F. Kelton, A. L. Greer, and C. V. Thompson, J. Chem. Phys. **79**, 6261 (1983).

[12] A. L. Biance, C. Clanet, and D. Quéré, Phys. Rev. E **69**, 016301 (2004).

[13] J. C. Bird, S. Mandre, and H. A. Stone, Phys. Rev. Lett. **100**, 234501 (2008).

[14] K. G. Winkels, J. H. Weijs, A. Eddi, and J. H. Snoeijer, Phys. Rev. E **85**, 55301 (2012).

[15] B. B. Stapelbroek, H. P. Jansen, E. S. Kooij, J. H. Snoeijer, and A. Eddi, Soft Matter **10**, 2641 (2014).

[16] L. H. Tanner, J. Phys. D **12**, 1473 (1979).
